# Supplementary material for: Learning the Travelling Salesperson Problem Requires Rethinking Generalization
Source: arXiv:2006.07054 source file (2022-05-25)
Supplement: Supplementary file 1 [file impact.tex]

Operations Research (OR) started in the first world war as an initiative to use mathematics and computer science to assist military planners in their decisions~\cite{gass2011history}.
Today, combinatorial optimization algorithms developed in the OR community form the backbone of the most important modern industries including transportation, logistics, scheduling, finance and supply chains.
However, designing powerful and robust optimization algorithms requires significant time and specialized knowledge, especially for understudied but high-impact problems arising in drug discovery~\cite{gomez2018automatic}, genomics~\cite{senior2020improved}, distributed systems~\cite{mao2019learning}, and circuit design~\cite{mirhoseini2020chip}.

In that respect, replacing domain experts and specialists with learning-based systems and data-driven approaches has had a `democratizing' effect in the broad algorithm design community~\cite{lecun2015deep,malik2017cvdl}. 
Today, tech-savy generalists and software engineers can deploy state-of-the-art solutions for challenging problems in computer vision~\cite{Girshick_2014_CVPR,dong2015image,he2016deep}, natural language~\cite{mikolov2013distributed,sutskever2014sequence,vaswani2017attention} and speech processing~\cite{oord2016wavenet,wang2017tacotron}.
We envision the long-term goal of end-to-end learning for combinatorial optimization to be similar: 
By making the modelling process intuitive for non-experts, learning-driven OR algorithms will be at the fingertips of more industries and can be personalized to individual users/use cases.

As an illustration, consider that you are a smartphone operating systems provider and want to optimize for battery life based on phone usage.
Instead of investing in expensive hardware specialists and years of R\&D,
on-device models driven by reinforcement learning algorithms such as the ones studied in this paper~\cite{bello2016neural,kool2018attention} can learn to optimize battery life in a personalized way from each individual phone's usage patterns.
However, unlike classical OR solvers which come with theoretical guarantees, our findings suggest that current learning-based approaches are not yet robust at handling situations beyond what they see in training and do not reliably scale to practical sizes.
Continuing our analogy, reinforcement learning models could eventually end up draining battery life faster if the architectures and policies are not robust or generalizable to, \textit{e.g.} low-cost and obscure smartphones which are often used by marginalized or low-income groups~\cite{samaan2003effect}.

This paper presents an initial technical investigation of these questions on the classical Travelling Salesman Problem, with the broader goal of developing robust and reliable learning-driven solvers for \textit{any} combinatorial problem.
TSP has a rich history of serving as an engine of discovery for general purpose techniques in applied mathematics, including foundational work in Mixed Integer Programming~\cite{dantzig1954solution}, Branch-and-bound methods~\cite{little1963algorithm}, heuristic search~\cite{aarts2003local} and early neural networks~\cite{hopfield1985neural,angeniol1988self}.
This line of work has already inspired novel reinforcement learning algorithms~\cite{kool2018attention} and powerful Graph Neural Network architectures~\cite{joshi2019efficient,dwivedi2020benchmarking}. 
Beyond combinatorial problems, designing statistical models that can generalize out-of-training-distribution is seen as an important challenge for the entire Machine Learning community~\cite{zhang2016understanding,finn2017model,bahdanau2018systematic,cobbe2018quantifying,Hill2020Environmental,lampinen2020transforming,linzen2020generalization}. 
In the near future, we hope TSP and combinatorial problems can serve as a challenging and practical benchmark for studying generalization in deep learning.
