# Supplementary material for: Learning the Travelling Salesperson Problem Requires Rethinking Generalization
Source: arXiv:2006.07054 source file (2022-05-25)
Supplement: Supplementary file 2 [file datasets.tex]

We generate 2D Euclidean TSP instances of varying sizes and complexities as graphs of $n$ node locations sampled uniformly in the unit square $S = \{x_i\}_{i=1}^n$ and $x_i \in {[0,1]}^2$.
For supervised learning, we generate a training set of 1,280,000 samples each for TSP20, TSP50, TSP100, and TSP20-50.
The groundtruth tours are obtained using the Concorde solver~\cite{applegate2006concorde}.
For reinforcement learning, 128,000 samples are randomly generated for each epoch (without optimal solutions).
We compare models on a held-out test set of 25,600 TSP samples and their corresponding optimal tours, consisting of 1,280 instances each of TSP10, TSP20, $\dots$, TSP200.
We release all our datasets as well as the associated scripts to produce TSP datasets of arbitrarily large sizes along with our open-source codebase.
